# Supplementary material for: Balanced Direction from Multifarious Choices: Arithmetic Meta-Learning for Domain Generalization
Source: arXiv:2503.18987 source file (2025-03-23)
Supplement: Supplementary file 1 [file _main.tex]

\clearpage
\setcounter{page}{1}
\maketitlesupplementary

\section{Proof of Gradient Matching}
\label{sec:appendix-a}

This section provides a detailed proof of gradient matching that
the gradient of step $k$ is matched with those of the previous $k$-1 steps.

\noindent \emph{Preliminary.} Let's start by revisiting the definitions of the inner loop of $n$ steps, during which the model's parameters transition from $\Theta$ to $\hat{\Theta}$. 
We represent the loss at each step as $\lbrace \mathcal{L}_1, \mathcal{L}_2, ..., \mathcal{L}_n\rbrace$, 
and the parameter updating trajectory as $\lbrace \theta_1, \theta_2, ..., \theta_{n+1}\rbrace$, with $\theta_1$ and $\theta_{n+1}$ corresponding to $\Theta$ and $\hat{\Theta}$ respectively.
We use $\mathcal{L}_i(\theta_j)$ to denote the loss of the $i$-th step on parameters $\theta_j$. 
During the inner loop, the update process is performed with a small learning rate $\alpha$: 
\begin{equation}
\label{eq:update-process}
\begin{split}
\theta_2 &= \theta_1 - \alpha\nabla\mathcal{L}_1(\theta_1) \\
\theta_3 &= \theta_2 - \alpha\nabla\mathcal{L}_2(\theta_2) \\
&\vdots  \\
\theta_{n+1} &= \theta_n - \alpha\nabla\mathcal{L}_n(\theta_n).
\end{split}
\end{equation}

\noindent \emph{Objective.} 
To prove that
% the gradient of any step is matched with those of the other $n$-1 steps, it is adequate to demonstrate that
for any $i=k$, step $k$ is gradient-matched with the previous $k$-1 steps as:
\begin{equation}
\label{eq:lossk-thetak}
\mathcal{L}_k(\theta_k) = \mathcal{L}_k(\theta_1) - \alpha\sum_{i=1}^{k-1}\nabla\mathcal{L}_i(\theta_1) \cdot \nabla\mathcal{L}_k(\theta_1) + \mathcal{O}(\alpha^2),
\end{equation}
% where gradient matching between two steps can be expressed by their dot product at $\theta_1$.
it is adequate to demonstrate that the following equation holds for any loss function $\mathcal{L}$:
\begin{equation}
\label{eq:loss-thetak}
\mathcal{L}(\theta_k) = \mathcal{L}(\theta_1) - \alpha\sum_{i=1}^{k-1}\nabla\mathcal{L}_i(\theta_1) \cdot \nabla\mathcal{L}(\theta_1) + \mathcal{O}(\alpha^2).
\end{equation}

\noindent \emph{Base Case.} When $i$ equals 1, it is evident that $\mathcal{L}(\theta_i) = \mathcal{L}(\theta_1)$, so \cref{eq:loss-thetak} holds. When $i$ equals 2, we can substitute \cref{eq:update-process} into $\mathcal{L}(\theta_2)$ and conduct a first order Taylor expansion on it: 
\begin{equation}
\label{eq:loss-theta2}
\mathcal{L}(\theta_2) = \mathcal{L}(\theta_1) - \alpha\nabla\mathcal{L}_1(\theta_1) \cdot \nabla\mathcal{L}(\theta_1) + \mathcal{O}(\alpha^2),
\end{equation}
thus \cref{eq:loss-thetak} is also valid.

\noindent \emph{Inductive Step.} Given that  \cref{eq:loss-thetak} is true for arbitrary $i \leq k$, we proceed to establish its validity for the case when $i$ equals $k+1$. 
Plugging \cref{eq:update-process} and \cref{eq:loss-thetak} into $\mathcal{L}(\theta_{k+1})$ yields:
\begin{equation}
\label{eq:loss-thetak+1}
\begin{split}
\mathcal{L}(\theta_{k+1}) =\ &\mathcal{L}(\theta_k) - \alpha\nabla\mathcal{L}_k(\theta_k) \cdot \nabla\mathcal{L}(\theta_k) + \mathcal{O}(\alpha^2) \\
=\ &\mathcal{L}(\theta_1) - \alpha\sum_{i=1}^{k-1}\nabla\mathcal{L}_i(\theta_1) \cdot \nabla\mathcal{L}(\theta_1) + \mathcal{O}(\alpha^2) \\
&- \alpha(\nabla\mathcal{L}_k(\theta_1) + \mathcal{O}(\alpha))(\nabla\mathcal{L}(\theta_1) + \mathcal{O}(\alpha)) + \mathcal{O}(\alpha^2) \\
=\ &\mathcal{L}(\theta_1) - \alpha\sum_{i=1}^{k}\nabla\mathcal{L}_i(\theta_1) \cdot \nabla\mathcal{L}(\theta_1) + \mathcal{O}(\alpha^2).
\end{split}
\end{equation}
Note that we substitute $\nabla\mathcal{L}_k(\theta_k)$ into \cref{eq:loss-thetak} to obtain: 
\begin{equation}
\label{eq:with-hessian}
\nabla\mathcal{L}_k(\theta_k) = \nabla\mathcal{L}_k(\theta_1) - \alpha\sum_{i=1}^{k-1}\nabla\mathcal{L}_i(\theta_1) \mathcal{H}_k(\theta_1) + \mathcal{O}(\alpha^2).
\end{equation}
$\mathcal{H}_k(\theta_1)$ is a Hessian left-multiplied by $\nabla\mathcal{L}_i(\theta_1)$.
\cref{eq:with-hessian} is simplified as $\nabla\mathcal{L}_k(\theta_1) + \mathcal{O}(\alpha)$ in \cref{eq:loss-thetak+1}, and $\nabla\mathcal{L}(\theta_k)$ follows the same process.

\vspace{0.05in}

\noindent \emph{Conclusion.} We have shown that \cref{eq:loss-thetak} is valid for all $i=k$ and for any loss function $\mathcal{L}$. Therefore, our objective of \cref{eq:lossk-thetak} is successfully demonstrated.

\section{Other Results.}
\label{sec:appendix-b}

We illustrate detailed results of Arith, as shown in \cref{tab:detailed}.
We also provide results from five datasets within the multi-modal WILDS benchmark \cite{koh2021wilds} as mentioned in main text. AMAZON, CAMELYON17 \cite{bandi2018detection}, CIVILCOMMENTS \cite{borkan2019nuanced}, IWILDCAM \cite{beery2020iwildcam}, and FMOW \cite{christie2018functional} present diverse challenges across multiple domains and modalities, and we adopt the hyperparameter configuration from \cite{shi2021gradient} to ensure consistency and comparability in our experiments.

\begin{itemize}
\item{AMAZON comprises 1.4 million customer reviews from 7,676 customers, with the goal of predicting a score (1-5 stars) for each review.}

\item{CAMELYON17 consists of 450,000 lymph node scans from five hospitals for cancer detection.}

\item{CIVILCOMMENTS includes 450,000 comments collected from online articles, each annotated for toxicity and mentions of demographic identities.}

\item{IWILDCAM contains over 200,000 wildlife photos captured by stationary cameras across 324 locations, aimed at identifying 186 species.}

\item{FMOW features satellite images from five regions over a span of 16 years, encompassing 62 categories.}
\end{itemize}

\clearpage
\section{Other Analysis.}
\label{sec:appendix-c}

\noindent \textbf{Why a balanced positioning?} The good balance refers to updating the model towards the centroid of domain experts, which integrates model averaging but differs in some key aspects (Sec. 2.5). 
This averaging can be viewed as a parameter-efficient form of ensemble learning, with a single model estimating the ensemble output of multiple domain experts. 
Consider a update trajectory $\lbrace \theta_1, \theta_2, ..., \theta_{n}\rbrace$, where 
$ \hat{\theta} = \frac{1}{n}\sum_{i=1}^n \theta_i$
and $f(\cdot)$ is the model's output. 
The Taylor expansion of the output ensemble is:
\begin{equation}  
\frac{1}{n}\sum_{i=1}^n f(\theta_i) = f(\hat{\theta}) + \frac{1}{n}\sum_{i=1}^n(\theta_i-\hat{\theta})^T \nabla f(\hat{\theta}) + \mathcal{O}(\alpha).
\end{equation}
The second term equals 0 because
$\sum_{i=1}^n(\theta_i-\hat{\theta}) = 0$, and
the third term is $\mathcal{O}(||\rm{max}_{i=1}^n(\theta_i-\hat{\theta})||^2)$. Along the same update trajectory, the different domain-optimal parameters are relatively close to each other, resulting in a smaller $(\theta_i-\hat{\theta})$, thus
$ f(\hat{\theta}) \approx \frac{1}{n}\sum_{i=1}^n f(\theta_i)$, indicating that our method closely estimates the ensemble output of domain experts.

\noindent \textbf{Discussion about computation and memory cost.} 
Our computation and memory costs are similar to other meta-learning methods. The computation cost primarily arises from backpropagation, which occurs only in the inner loop that we do not modify, thus keeping this cost comparable to other methods. Although increasing the number of steps raises costs, all comparisons are conducted with the same number of steps. For example, the training time for Fish and our method with 5000 iterations on the PACS dataset is 85.4 \emph{min} and 91.9 \emph{min}, respectively.
The main memory cost is due to the computation graph generated by backpropagation.
Our method continuously accumulates the gradients during the inner loop to update parameters without generating additional computation graphs. As a result, the extra memory overhead is limited to storing these gradients, which is no larger than the size of the model's inherent parameters. For example, it is 90M for ResNet50, which is negligible compared to the total cost of approximately 6000M with a batch size of 32 for three domains.
{
    \small
    \bibliographystyle{ieeenat_fullname}
    \bibliography{main}
}
\clearpage
\begin{table*}[h]
% \renewcommand\arraystretch{1}
% \small
\caption{Detailed results on DomainBed benchmark.}
\vspace{-0.05in}
\centering
\begin{tabular}{c|ccccc}
\toprule
\textbf{Domain Index} & \textbf{PACS} & \textbf{VLCS} & \textbf{OfficeH} & \textbf{TerraInc} & \textbf{DomainNet} \\
\midrule
Domain 1 & 85.9 \tiny{$\pm$ 0.5} & 98.7 \tiny{$\pm$ 0.3} & 64.6 \tiny{$\pm$ 0.8} & 52.3 \tiny{$\pm$ 1.9} & 59.0 \tiny{$\pm$ 0.4} \\
Domain 2 & 81.3 \tiny{$\pm$ 1.0} & 64.3 \tiny{$\pm$ 0.8} & 55.3 \tiny{$\pm$ 0.9} & 42.4 \tiny{$\pm$ 2.5} & 19.7 \tiny{$\pm$ 0.2} \\
Domain 3 & 97.1 \tiny{$\pm$ 0.5} & 76.0 \tiny{$\pm$ 0.9} & 78.3 \tiny{$\pm$ 0.4} & 57.5 \tiny{$\pm$ 1.3} & 47.0 \tiny{$\pm$ 0.3} \\
Domain 4 & 81.8 \tiny{$\pm$ 1.0} & 78.6 \tiny{$\pm$ 1.0} & 79.4 \tiny{$\pm$ 0.6} & 40.2 \tiny{$\pm$ 2.3} & 12.7 \tiny{$\pm$ 0.3} \\
Domain 5 & - & - & - & - & 59.4 \tiny{$\pm$ 0.4} \\
Domain 6 & - & - & - & - & 51.1 \tiny{$\pm$ 0.7} \\

\midrule

Avg & 86.5 \tiny{$\pm$ 0.3} & 79.4 \tiny{$\pm$ 0.3} & 69.4 \tiny{$\pm$ 0.1} & 48.1 \tiny{$\pm$ 1.2} & 41.5 \tiny{$\pm$ 0.1} \\
\bottomrule
\end{tabular}
\vspace{0.1in}
\label{tab:detailed}
\end{table*}

\begin{table*}[h]
% \renewcommand\arraystretch{1}
% \small
\caption{Results on AMAZON (\%)}
\vspace{-0.05in}
\centering
\begin{tabular}{c|ccc}
\toprule
\textbf{Method} & \textbf{Average acc} & \textbf{10th acc} & \textbf{Worst acc} \\
\midrule

ERM & 70.3 & 50.7 & 4.0 \\
Fish & 70.6 & 51.1 & 5.3 \\
Arith & \textbf{70.7} & \textbf{52.0} & \textbf{5.3} \\

\bottomrule
\end{tabular}
\vspace{0.1in}
\label{tab:amazon}
\end{table*}

\begin{table*}[h]
% \renewcommand\arraystretch{1}
% \small
\caption{Accuracy on CAMELYON17 (\%)}
\vspace{-0.05in}
\centering
\begin{tabular}{c|ccccccccccc}
\toprule
\textbf{Method} & \textbf{20} & \textbf{21} & \textbf{22} & \textbf{23} & \textbf{24} & \textbf{25} & \textbf{26} & \textbf{27} & \textbf{28} & \textbf{29} & \textbf{Avg} \\
\midrule
ERM & 49.2 & 30.2 & 73.6 & 74.8 & 64.4 & 60.8 & 57.0 & 37.8 & 89.6 & 77.3 & 73.1 \\
Fish & 52.4 & \textbf{36.0} & 72.3 & \textbf{77.5} & 69.0 & 65.1 & 59.3 & \textbf{43.6} & 90.0 & 77.6 & 74.8 \\
Arith & \textbf{54.4} & 33.8 & \textbf{83.6} & 75.2 & \textbf{72.5} & \textbf{69.5} & \textbf{64.0} & 40.7 & \textbf{90.1} & \textbf{79.9} & \textbf{76.6} \\

\bottomrule
\end{tabular}
\vspace{0.1in}
\label{tab:camelyon17}
\end{table*}

\begin{table*}[h]
% \renewcommand\arraystretch{1}
% \small
\caption{Accuracy on CIVILCOMMENTS (\%)}
\vspace{-0.05in}
\centering
\resizebox{1\linewidth}{!}{
\begin{tabular}{c|ccccccccccccccccc}
\toprule
\textbf{Method} & \textbf{N1} & \textbf{N2} & \textbf{N3} & \textbf{N4} & \textbf{N5} & \textbf{N6} & \textbf{N7} & \textbf{N8} & \textbf{T1} & \textbf{T2} & \textbf{T3} & \textbf{T4} & \textbf{T5} & \textbf{T6} & \textbf{T7} & \textbf{T8} & \textbf{Avg} \\
\midrule

ERM & 82.8 & 84.4 & 72.0 & 89.9 & 77.8 & 83.8 & 70.5 & 71.2 & \textbf{82.7} & \textbf{82.8} & \textbf{78.7} & \textbf{79.0} & \textbf{77.1} & 76.1 & 80.7 & 80.5 & 87.4 \\

Fish & 84.9 & 86.4 & 76.8 & 90.6 & \textbf{80.9} & \textbf{85.5} & 72.5 & \textbf{73.9} & 79.8 & 79.9 & 73.2 & 76.5 & 74.1 & 76.3 & 80.1 & 79.6 & 87.9 \\

Arith & \textbf{87.8} & \textbf{89.3} & \textbf{77.9} & \textbf{91.5} & 80.6 & 85.4 & \textbf{73.5} & 72.1 & 77.3 & 76.1 & 73.2 & 75.0 & 74.8 & \textbf{77.1} & \textbf{80.9} & \textbf{81.1} & \textbf{90.0} \\

\bottomrule
\end{tabular}
}
\vspace{0.1in}
\label{tab:civil}
\end{table*}

\begin{table*}[h]
% \renewcommand\arraystretch{1}
% \small
\caption{Results on IWILDCAM (\%)}
\vspace{-0.05in}
\centering
\begin{tabular}{c|ccc}
\toprule
\textbf{Method} & \textbf{Average acc} & \textbf{Recall macro} & \textbf{F1 macro} \\
\midrule

ERM & 61.6 & 23.4 & 20.7 \\
Fish & 62.2 & 22.7 & 21.1 \\
Arith & \textbf{63.2} & \textbf{25.2} & \textbf{22.5} \\ 

\bottomrule
\end{tabular}
\vspace{0.1in}
\label{tab:iwildcam}
\end{table*}

\begin{table*}[h]
% \renewcommand\arraystretch{1}
% \small
\caption{Accuracy on FMOW (\%)}
\vspace{-0.05in}
\centering
\begin{tabular}{c|cccccccc}
\toprule
\textbf{Method} & \textbf{2016} & \textbf{2017} & \textbf{Asi} & \textbf{Eur} & \textbf{Afr} & \textbf{Ame} & \textbf{Oce} & \textbf{Avg} \\
\midrule

ERM & 53.4 & 47.0 & 51.9 & 54.8 & 33.3 & 54.4 & 58.7 & 51.6 \\
Fish & 53.7 & 47.5 & 52.7 & \textbf{55.0} & 33.9 & \textbf{54.6} & \textbf{59.0} & 52.0 \\
Arith & \textbf{53.8} & \textbf{47.9} & \textbf{54.5} & 54.8 & \textbf{34.1} & 54.2 & 57.2 & \textbf{52.2}\\

\bottomrule
\end{tabular}

\vspace{0.1in}
\label{tab:fmow}
\end{table*}
