# Supplementary material for: Balanced Direction from Multifarious Choices: Arithmetic Meta-Learning for Domain Generalization
Source: arXiv:2503.18987 source file (2025-03-23)
Supplement: Supplementary file 3 [file 01_proof.tex]

\section{Proof of Gradient Matching}
\label{sec:appendix-a}

This section provides a detailed proof of gradient matching that
the gradient of step $k$ is matched with those of the previous $k$-1 steps.

\noindent \emph{Preliminary.} Let's start by revisiting the definitions of the inner loop of $n$ steps, during which the model's parameters transition from $\Theta$ to $\hat{\Theta}$. 
We represent the loss at each step as $\lbrace \mathcal{L}_1, \mathcal{L}_2, ..., \mathcal{L}_n\rbrace$, 
and the parameter updating trajectory as $\lbrace \theta_1, \theta_2, ..., \theta_{n+1}\rbrace$, with $\theta_1$ and $\theta_{n+1}$ corresponding to $\Theta$ and $\hat{\Theta}$ respectively.
We use $\mathcal{L}_i(\theta_j)$ to denote the loss of the $i$-th step on parameters $\theta_j$. 
During the inner loop, the update process is performed with a small learning rate $\alpha$: 
\begin{equation}
\label{eq:update-process}
\begin{split}
\theta_2 &= \theta_1 - \alpha\nabla\mathcal{L}_1(\theta_1) \\
\theta_3 &= \theta_2 - \alpha\nabla\mathcal{L}_2(\theta_2) \\
&\vdots  \\
\theta_{n+1} &= \theta_n - \alpha\nabla\mathcal{L}_n(\theta_n).
\end{split}
\end{equation}

\noindent \emph{Objective.} 
To prove that
% the gradient of any step is matched with those of the other $n$-1 steps, it is adequate to demonstrate that
for any $i=k$, step $k$ is gradient-matched with the previous $k$-1 steps as:
\begin{equation}
\label{eq:lossk-thetak}
\mathcal{L}_k(\theta_k) = \mathcal{L}_k(\theta_1) - \alpha\sum_{i=1}^{k-1}\nabla\mathcal{L}_i(\theta_1) \cdot \nabla\mathcal{L}_k(\theta_1) + \mathcal{O}(\alpha^2),
\end{equation}
% where gradient matching between two steps can be expressed by their dot product at $\theta_1$.
it is adequate to demonstrate that the following equation holds for any loss function $\mathcal{L}$:
\begin{equation}
\label{eq:loss-thetak}
\mathcal{L}(\theta_k) = \mathcal{L}(\theta_1) - \alpha\sum_{i=1}^{k-1}\nabla\mathcal{L}_i(\theta_1) \cdot \nabla\mathcal{L}(\theta_1) + \mathcal{O}(\alpha^2).
\end{equation}

\noindent \emph{Base Case.} When $i$ equals 1, it is evident that $\mathcal{L}(\theta_i) = \mathcal{L}(\theta_1)$, so \cref{eq:loss-thetak} holds. When $i$ equals 2, we can substitute \cref{eq:update-process} into $\mathcal{L}(\theta_2)$ and conduct a first order Taylor expansion on it: 
\begin{equation}
\label{eq:loss-theta2}
\mathcal{L}(\theta_2) = \mathcal{L}(\theta_1) - \alpha\nabla\mathcal{L}_1(\theta_1) \cdot \nabla\mathcal{L}(\theta_1) + \mathcal{O}(\alpha^2),
\end{equation}
thus \cref{eq:loss-thetak} is also valid.

\noindent \emph{Inductive Step.} Given that  \cref{eq:loss-thetak} is true for arbitrary $i \leq k$, we proceed to establish its validity for the case when $i$ equals $k+1$. 
Plugging \cref{eq:update-process} and \cref{eq:loss-thetak} into $\mathcal{L}(\theta_{k+1})$ yields:
\begin{equation}
\label{eq:loss-thetak+1}
\begin{split}
\mathcal{L}(\theta_{k+1}) =\ &\mathcal{L}(\theta_k) - \alpha\nabla\mathcal{L}_k(\theta_k) \cdot \nabla\mathcal{L}(\theta_k) + \mathcal{O}(\alpha^2) \\
=\ &\mathcal{L}(\theta_1) - \alpha\sum_{i=1}^{k-1}\nabla\mathcal{L}_i(\theta_1) \cdot \nabla\mathcal{L}(\theta_1) + \mathcal{O}(\alpha^2) \\
&- \alpha(\nabla\mathcal{L}_k(\theta_1) + \mathcal{O}(\alpha))(\nabla\mathcal{L}(\theta_1) + \mathcal{O}(\alpha)) + \mathcal{O}(\alpha^2) \\
=\ &\mathcal{L}(\theta_1) - \alpha\sum_{i=1}^{k}\nabla\mathcal{L}_i(\theta_1) \cdot \nabla\mathcal{L}(\theta_1) + \mathcal{O}(\alpha^2).
\end{split}
\end{equation}
Note that we substitute $\nabla\mathcal{L}_k(\theta_k)$ into \cref{eq:loss-thetak} to obtain: 
\begin{equation}
\label{eq:with-hessian}
\nabla\mathcal{L}_k(\theta_k) = \nabla\mathcal{L}_k(\theta_1) - \alpha\sum_{i=1}^{k-1}\nabla\mathcal{L}_i(\theta_1) \mathcal{H}_k(\theta_1) + \mathcal{O}(\alpha^2).
\end{equation}
$\mathcal{H}_k(\theta_1)$ is a Hessian left-multiplied by $\nabla\mathcal{L}_i(\theta_1)$.
\cref{eq:with-hessian} is simplified as $\nabla\mathcal{L}_k(\theta_1) + \mathcal{O}(\alpha)$ in \cref{eq:loss-thetak+1}, and $\nabla\mathcal{L}(\theta_k)$ follows the same process.

\vspace{0.05in}

\noindent \emph{Conclusion.} We have shown that \cref{eq:loss-thetak} is valid for all $i=k$ and for any loss function $\mathcal{L}$. Therefore, our objective of \cref{eq:lossk-thetak} is successfully demonstrated.
