# Supplementary material for: Balanced Direction from Multifarious Choices: Arithmetic Meta-Learning for Domain Generalization
Source: arXiv:2503.18987 source file (2025-03-23)
Supplement: Supplementary file 4 [file 02_results.tex]

\section{Other Results.}
\label{sec:appendix-b}

We illustrate detailed results of Arith, as shown in \cref{tab:detailed}.
We also provide results from five datasets within the multi-modal WILDS benchmark \cite{koh2021wilds} as mentioned in main text. AMAZON, CAMELYON17 \cite{bandi2018detection}, CIVILCOMMENTS \cite{borkan2019nuanced}, IWILDCAM \cite{beery2020iwildcam}, and FMOW \cite{christie2018functional} present diverse challenges across multiple domains and modalities, and we adopt the hyperparameter configuration from \cite{shi2021gradient} to ensure consistency and comparability in our experiments.

\begin{itemize}
\item{AMAZON comprises 1.4 million customer reviews from 7,676 customers, with the goal of predicting a score (1-5 stars) for each review.}

\item{CAMELYON17 consists of 450,000 lymph node scans from five hospitals for cancer detection.}

\item{CIVILCOMMENTS includes 450,000 comments collected from online articles, each annotated for toxicity and mentions of demographic identities.}

\item{IWILDCAM contains over 200,000 wildlife photos captured by stationary cameras across 324 locations, aimed at identifying 186 species.}

\item{FMOW features satellite images from five regions over a span of 16 years, encompassing 62 categories.}
\end{itemize}
