# Supplementary material for: Balanced Direction from Multifarious Choices: Arithmetic Meta-Learning for Domain Generalization
Source: arXiv:2503.18987 source file (2025-03-23)
Supplement: Supplementary file 5 [file 03_costs.tex]

\clearpage
\section{Other Analysis.}
\label{sec:appendix-c}

\noindent \textbf{Why a balanced positioning?} The good balance refers to updating the model towards the centroid of domain experts, which integrates model averaging but differs in some key aspects (Sec. 2.5). 
This averaging can be viewed as a parameter-efficient form of ensemble learning, with a single model estimating the ensemble output of multiple domain experts. 
Consider a update trajectory $\lbrace \theta_1, \theta_2, ..., \theta_{n}\rbrace$, where 
$ \hat{\theta} = \frac{1}{n}\sum_{i=1}^n \theta_i$
and $f(\cdot)$ is the model's output. 
The Taylor expansion of the output ensemble is:
\begin{equation}  
\frac{1}{n}\sum_{i=1}^n f(\theta_i) = f(\hat{\theta}) + \frac{1}{n}\sum_{i=1}^n(\theta_i-\hat{\theta})^T \nabla f(\hat{\theta}) + \mathcal{O}(\alpha).
\end{equation}
The second term equals 0 because
$\sum_{i=1}^n(\theta_i-\hat{\theta}) = 0$, and
the third term is $\mathcal{O}(||\rm{max}_{i=1}^n(\theta_i-\hat{\theta})||^2)$. Along the same update trajectory, the different domain-optimal parameters are relatively close to each other, resulting in a smaller $(\theta_i-\hat{\theta})$, thus
$ f(\hat{\theta}) \approx \frac{1}{n}\sum_{i=1}^n f(\theta_i)$, indicating that our method closely estimates the ensemble output of domain experts.

\noindent \textbf{Discussion about computation and memory cost.} 
Our computation and memory costs are similar to other meta-learning methods. The computation cost primarily arises from backpropagation, which occurs only in the inner loop that we do not modify, thus keeping this cost comparable to other methods. Although increasing the number of steps raises costs, all comparisons are conducted with the same number of steps. For example, the training time for Fish and our method with 5000 iterations on the PACS dataset is 85.4 \emph{min} and 91.9 \emph{min}, respectively.
The main memory cost is due to the computation graph generated by backpropagation.
Our method continuously accumulates the gradients during the inner loop to update parameters without generating additional computation graphs. As a result, the extra memory overhead is limited to storing these gradients, which is no larger than the size of the model's inherent parameters. For example, it is 90M for ResNet50, which is negligible compared to the total cost of approximately 6000M with a batch size of 32 for three domains.
