# Supplementary material for: Balanced Direction from Multifarious Choices: Arithmetic Meta-Learning for Domain Generalization
Source: arXiv:2503.18987 source file (2025-03-23)
Supplement: Supplementary file 6 [file 04_tables.tex]

\begin{table*}[h]
% \renewcommand\arraystretch{1}
% \small
\caption{Detailed results on DomainBed benchmark.}
\vspace{-0.05in}
\centering
\begin{tabular}{c|ccccc}
\toprule
\textbf{Domain Index} & \textbf{PACS} & \textbf{VLCS} & \textbf{OfficeH} & \textbf{TerraInc} & \textbf{DomainNet} \\
\midrule
Domain 1 & 85.9 \tiny{$\pm$ 0.5} & 98.7 \tiny{$\pm$ 0.3} & 64.6 \tiny{$\pm$ 0.8} & 52.3 \tiny{$\pm$ 1.9} & 59.0 \tiny{$\pm$ 0.4} \\
Domain 2 & 81.3 \tiny{$\pm$ 1.0} & 64.3 \tiny{$\pm$ 0.8} & 55.3 \tiny{$\pm$ 0.9} & 42.4 \tiny{$\pm$ 2.5} & 19.7 \tiny{$\pm$ 0.2} \\
Domain 3 & 97.1 \tiny{$\pm$ 0.5} & 76.0 \tiny{$\pm$ 0.9} & 78.3 \tiny{$\pm$ 0.4} & 57.5 \tiny{$\pm$ 1.3} & 47.0 \tiny{$\pm$ 0.3} \\
Domain 4 & 81.8 \tiny{$\pm$ 1.0} & 78.6 \tiny{$\pm$ 1.0} & 79.4 \tiny{$\pm$ 0.6} & 40.2 \tiny{$\pm$ 2.3} & 12.7 \tiny{$\pm$ 0.3} \\
Domain 5 & - & - & - & - & 59.4 \tiny{$\pm$ 0.4} \\
Domain 6 & - & - & - & - & 51.1 \tiny{$\pm$ 0.7} \\

\midrule

Avg & 86.5 \tiny{$\pm$ 0.3} & 79.4 \tiny{$\pm$ 0.3} & 69.4 \tiny{$\pm$ 0.1} & 48.1 \tiny{$\pm$ 1.2} & 41.5 \tiny{$\pm$ 0.1} \\
\bottomrule
\end{tabular}
\vspace{0.1in}
\label{tab:detailed}
\end{table*}

\begin{table*}[h]
% \renewcommand\arraystretch{1}
% \small
\caption{Results on AMAZON (\%)}
\vspace{-0.05in}
\centering
\begin{tabular}{c|ccc}
\toprule
\textbf{Method} & \textbf{Average acc} & \textbf{10th acc} & \textbf{Worst acc} \\
\midrule

ERM & 70.3 & 50.7 & 4.0 \\
Fish & 70.6 & 51.1 & 5.3 \\
Arith & \textbf{70.7} & \textbf{52.0} & \textbf{5.3} \\

\bottomrule
\end{tabular}
\vspace{0.1in}
\label{tab:amazon}
\end{table*}

\begin{table*}[h]
% \renewcommand\arraystretch{1}
% \small
\caption{Accuracy on CAMELYON17 (\%)}
\vspace{-0.05in}
\centering
\begin{tabular}{c|ccccccccccc}
\toprule
\textbf{Method} & \textbf{20} & \textbf{21} & \textbf{22} & \textbf{23} & \textbf{24} & \textbf{25} & \textbf{26} & \textbf{27} & \textbf{28} & \textbf{29} & \textbf{Avg} \\
\midrule
ERM & 49.2 & 30.2 & 73.6 & 74.8 & 64.4 & 60.8 & 57.0 & 37.8 & 89.6 & 77.3 & 73.1 \\
Fish & 52.4 & \textbf{36.0} & 72.3 & \textbf{77.5} & 69.0 & 65.1 & 59.3 & \textbf{43.6} & 90.0 & 77.6 & 74.8 \\
Arith & \textbf{54.4} & 33.8 & \textbf{83.6} & 75.2 & \textbf{72.5} & \textbf{69.5} & \textbf{64.0} & 40.7 & \textbf{90.1} & \textbf{79.9} & \textbf{76.6} \\

\bottomrule
\end{tabular}
\vspace{0.1in}
\label{tab:camelyon17}
\end{table*}

\begin{table*}[h]
% \renewcommand\arraystretch{1}
% \small
\caption{Accuracy on CIVILCOMMENTS (\%)}
\vspace{-0.05in}
\centering
\resizebox{1\linewidth}{!}{
\begin{tabular}{c|ccccccccccccccccc}
\toprule
\textbf{Method} & \textbf{N1} & \textbf{N2} & \textbf{N3} & \textbf{N4} & \textbf{N5} & \textbf{N6} & \textbf{N7} & \textbf{N8} & \textbf{T1} & \textbf{T2} & \textbf{T3} & \textbf{T4} & \textbf{T5} & \textbf{T6} & \textbf{T7} & \textbf{T8} & \textbf{Avg} \\
\midrule

ERM & 82.8 & 84.4 & 72.0 & 89.9 & 77.8 & 83.8 & 70.5 & 71.2 & \textbf{82.7} & \textbf{82.8} & \textbf{78.7} & \textbf{79.0} & \textbf{77.1} & 76.1 & 80.7 & 80.5 & 87.4 \\

Fish & 84.9 & 86.4 & 76.8 & 90.6 & \textbf{80.9} & \textbf{85.5} & 72.5 & \textbf{73.9} & 79.8 & 79.9 & 73.2 & 76.5 & 74.1 & 76.3 & 80.1 & 79.6 & 87.9 \\

Arith & \textbf{87.8} & \textbf{89.3} & \textbf{77.9} & \textbf{91.5} & 80.6 & 85.4 & \textbf{73.5} & 72.1 & 77.3 & 76.1 & 73.2 & 75.0 & 74.8 & \textbf{77.1} & \textbf{80.9} & \textbf{81.1} & \textbf{90.0} \\

\bottomrule
\end{tabular}
}
\vspace{0.1in}
\label{tab:civil}
\end{table*}

\begin{table*}[h]
% \renewcommand\arraystretch{1}
% \small
\caption{Results on IWILDCAM (\%)}
\vspace{-0.05in}
\centering
\begin{tabular}{c|ccc}
\toprule
\textbf{Method} & \textbf{Average acc} & \textbf{Recall macro} & \textbf{F1 macro} \\
\midrule

ERM & 61.6 & 23.4 & 20.7 \\
Fish & 62.2 & 22.7 & 21.1 \\
Arith & \textbf{63.2} & \textbf{25.2} & \textbf{22.5} \\ 

\bottomrule
\end{tabular}
\vspace{0.1in}
\label{tab:iwildcam}
\end{table*}

\begin{table*}[h]
% \renewcommand\arraystretch{1}
% \small
\caption{Accuracy on FMOW (\%)}
\vspace{-0.05in}
\centering
\begin{tabular}{c|cccccccc}
\toprule
\textbf{Method} & \textbf{2016} & \textbf{2017} & \textbf{Asi} & \textbf{Eur} & \textbf{Afr} & \textbf{Ame} & \textbf{Oce} & \textbf{Avg} \\
\midrule

ERM & 53.4 & 47.0 & 51.9 & 54.8 & 33.3 & 54.4 & 58.7 & 51.6 \\
Fish & 53.7 & 47.5 & 52.7 & \textbf{55.0} & 33.9 & \textbf{54.6} & \textbf{59.0} & 52.0 \\
Arith & \textbf{53.8} & \textbf{47.9} & \textbf{54.5} & 54.8 & \textbf{34.1} & 54.2 & 57.2 & \textbf{52.2}\\

\bottomrule
\end{tabular}

\vspace{0.1in}
\label{tab:fmow}
\end{table*}
